# Supplementary material for: Two mixed finite element formulations for the weak imposition of the Neumann boundary conditions for the Darcy flow
Source: arXiv:2104.01366 source file (2021-04-03)
Supplement: Supplementary file 1 [file appendix.tex]

\section{Auxiliary theoretical results}
For the sake of completeness, let us recall the definition of a Lipschitz domain which, loosely speaking, requires the domain to be locally the epigraph of a Lipschitz function.
\begin{definition}
$\Omega\subset\R^d$ open and bounded is said to be \emph{Lipschitz} if for every $x_0\in\partial\Omega$	there exists $r>0$ and $\gamma: \R^{n-1}\to\R$ Lipschitz such that, upon relabelling and reorienting the coordinate axes if necessary,
\begin{equation*}
B(x_0,r)\cap\Omega=\{x=\left(x_1,\dots,x_d\right)\in\R^d: x_d>\gamma(x_1,\dots,x_{d-1})\}.
\end{equation*}
\end{definition}	

\begin{lemma}\label{lemma:disc_trace_ineq}
	There exists $C>0$ depending on $\Gamma_N$, but not on the way it cuts the mesh, such that for every $K\in\mathcal G_h$:
	\begin{equation*}
		\norm{v}^2_{L^2(\Gamma_K)}\le C_T \norm{v}_{L^2(K)}\norm{\nabla v}_{L^2(K)}\qquad\forall\ v\in H^1(K).
	\end{equation*}	
\end{lemma}	
\begin{proof}
	See, for instance, Lemma 3 in~\cite{Hansbo434217}.
\end{proof}	

\begin{lemma}\label{lemma:poly1}
Let $K,K'\in\mathcal T_h$ be such that $K'\in\mathcal N(K)$. There exists $C>0$ such that
\begin{equation*}
\norm{p}_{L^\infty(K)}\le C\norm{p}_{L^\infty(K')}\qquad\forall\ p\in\mathbb{Q}_k(\R^d),
\end{equation*}
where $C$ depends on $k$ and on the shape regularity of the mesh.
\end{lemma}
\begin{proof}
The proof easily follows by a scaling argument. See Lemma A.3 in~\cite{puppi}.
\end{proof}
%\begin{proof}
%We define
%\begin{equation*}
%\begin{aligned}
%&\psi:\R^N\setminus\{ 0\}\to\mathbb{R} \\
%&\psi(\boldsymbol{\eta})=\frac{\norm{p}_{L^\infty(Q)}}{\norm{p}_{L^\infty(Q')}}=\frac{\max_{x\in Q}\abs{\sum_{i=1}^N\eta_i\varphi_i}}{\max_{x\in Q'}\abs{\sum_{i=1}^N\eta_i\varphi_i}},
%\end{aligned}
%\end{equation*}
%where $\boldsymbol{\eta}$ are the coordinates of $p$ with respect to the basis $\{\varphi_i \}_{i=1,\dots, N}$. Note that $\psi$ is continuous and homogeneous of degree $0$, i.e. $\psi(t\boldsymbol{\eta})=\psi(\boldsymbol{\eta})$ $\forall\ t>0$. In particular, by homogeneity
%\begin{equation*}
%\psi\left(\boldsymbol{\eta}\right) =\psi\left( \abs{\boldsymbol{\eta}}_{\R^{N_h}}\frac{\boldsymbol{\eta}}{\abs{\boldsymbol{\eta}}}_{\R^{N_h}}\right) = \psi\left(\frac{\boldsymbol{\eta}}{\abs{\boldsymbol{\eta}}_{\R^{N_h}}}\right),
%\end{equation*}
%that is $\psi$ is determined by its values on the unit sphere
%\begin{equation*}
%S=\{\boldsymbol{\eta}\in\R^N:\abs{\boldsymbol{\eta}}_{\R^{N_h}}=1\}
%\end{equation*}
%which is compact. By Weierstrass theorem $\psi$ attains its maximum on $S$, i.e. there exists $C>0$ such that
%\begin{equation*}
%\abs{\psi(\boldsymbol{\eta})}\le C.
%\end{equation*}
%Note that $C$ depends on the dimension $N$ (i.e. on the degree $k=N-1$), on the shape regularity of the mesh and on the distance between $Q$ and $Q'$ (we are evaluating the same basis functions $\{\varphi_i \}_{i=1,\dots, N}$ at points which are far from each other). Since we are supposing $Q,Q'$ neighbours we do not have the last dependency.
%\end{proof}

The next one says that the $L^2$ norm on the cut portion of an element $K$ controls the $L^\infty$ (and hence any other) norm on the whole element with an equivalence constant depending on the relative measure of the cut portion.
\begin{lemma}\label{lemma:poly2}
Let $0<\theta\le 1$. There exists $C>0$ such that for every $K\in\mathcal T_h$ and every $S\subset K$ measurable such that $\abs{S}\ge \theta\abs{K}$, we have
\begin{equation*}
\norm{p}_{L^\infty(K)}\le C h_{\min}^{-\frac{d}{2}}\norm{p}_{L^2(S)}\qquad\forall\ p\in\mathbb{Q}_k(\R^d),
\end{equation*}
where $C$ depends only on $\theta$, $k$ and the mesh regularity.
\end{lemma}
\begin{proof}
See Proposition 1 in \cite{lozinski}. 
\end{proof}
